# Supplementary material for: Hidden Gems: 4D Radar Scene Flow Learning Using Cross-Modal Supervision
Source: arXiv:2303.00462 source file (2023-03-17)
Supplement: Supplementary file 1 [file supplementary.tex]

\newpage
\section{Supplementary Materials}
\label{sec:supp}

\subsection{Dataset Details.}
\noindent\textbf{Dataset separation.}
For evaluation, we split the VoD dataset~\cite{palffy2022multi} ourselves in our experiments. In our new separation, we kept the original \emph{Val} set unchanged and divide a part of the original training set into a new \emph{Test} set so that we can generate ground truth scene flow for evaluation. The left sequences from the original training set make up a new $\emph{Train}~(A)$ set. As this set have annotated labels, we can use it for fully-supervised learning methods. To avoid wasting the data from the original testing set, we combine it with our new $\emph{Train}~(A)$ set into a larger $\emph{Train}$ set. We remove the annotated labels from the $\emph{Train}~(A)$ set for this set and only use it for self-supervised or cross-modal supervised learning methods.

\noindent\textbf{Data preprocessing.} Given sequences of radar point clouds, we first filter out the radar points outside the Field-of-View (FoV) of camera as only objects partially or fully with the camera FoV are annotated.  Then, we set a z-axis range [-3m, 3m] and filter points outside the range (usually outliers). In the training sequence, we randomly sample 256 radar points for each point cloud to facilitate fast mini-batch learning.  For point clouds used for inference, we keep the original number of points because our task is to estimate the flow vector of each radar point. Finally, we form $L_{seq}-1$ scene flow input samples for each sequence by combining pairs of consecutive radar point clouds, where $L_{seq}$ is the length of the sequence. 

\noindent\textbf{Ground truth labelling.} Following~\cite{jund2021scalable, baur2021slim}, we annotate ground truth scene flow with ground truth object annotations and radar ego-motion. For points belonging to the static background, we label their flow vectors with the ground truth radar ego-motion. For the foreground objects, we track the ID of each annotated bounding box across consecutive point clouds and compute their rigid transformation w.r.t the radar coordinate frame. Each foreground point are assigned a ground truth flow vector summarized by its corresponding rigid transformation. To obtain the ground truth motion segmentation, we compensate radar ego-motion for the flow vector of each foreground point and label points whose non-rigid flow larger than 5cm as moving, while the rest points are labelled as static.

\subsection{Model Architecture Details.}
Here, we introduce more detailed module design, layer hyperparameters of our model architecture. 

\noindent\textbf{Backbone.} The input to our backbone is two consecutive 4D radar point clouds, $\mathbf{P}^{s}\in\mathbb{R}^{N\times({3+C})}$ and $\mathbf{P}^{t}\in\mathbb{R}^{M\times({3+C})}$. As the foremost step, we use four \emph{set conv} layers~\cite{liu2019flownet3d} to extract local features at different scales. Detailed layer parameters of this multi-scale \emph{set conv} layer are as follows:
\begin{flalign*}
& \textrm{syntax:}~{SC ([radii], [nsamples], [dimension])} &
\end{flalign*}
\vspace{-2em}
\begin{flalign*}
& SC ([2.0, 4.0, 8.0, 16.0], [4, 8, 16, 32], 
[[32,32,64], [32, 32, \\
& 64], [32, 32, 64], [32, 32, 64]])\rightarrow MLP (256\rightarrow256)
\end{flalign*}
where $[radii]$ denotes the grouping radii for multiple scales, $[nsamples]$ denotes the number of local sampled points, $[dimension]$ are the latent feature dimensions. Note that we do not downsample our sparse radar point clouds. After concatenating global feature vector to  point-wise features, we obtain the local-global features for each individual input point cloud,  $g_{\theta}(\mathbf{P}^{s})\in\mathbb{R}^{N\times 512}$ and $g_{\theta}(\mathbf{P}^{t})\in\mathbb{R}^{M\times 512}$.

To propagate the feature from the target point cloud to the source, we adopt the \emph{cost volume} layer~\cite{wu2020pointpwc} to compute pair-wise costs and aggregate them in a robust patch-to-patch manner. For cost computation, detailed hyperparameters are:
\begin{flalign*}
& MLP (512\times 2 + 3\rightarrow 512\rightarrow 512 \rightarrow 512)
\end{flalign*}
In patch-to-patch cost aggregation, the number of neighbour points are set to be 8. As a results, we can obtain the correlated features $h_{\theta}(g_{\theta}(\mathbf{P}^{s}), g_{\theta}(\mathbf{P}^{t}))\in\mathbb{R}^{N\times 512}$. 

The flow embedding $FE\in\mathbb{R}^{N\times (512+512+C)}$ can be generated by concatenating the correlated features, the local-global features and the raw input features of $\mathbf{P}^{s}$. We further feed this flow embedding into another multi-scale \emph{set conv} layer to get $\mathbf{L}\in\mathbb{R}^{N\times 256}$:  
\begin{flalign*}
& SC ([2.0, 4.0, 8.0, 16.0], [4, 8, 16, 32], 
[[512,256,64], \\
& [512, 256, 64], [512,256,64], [512,256,64]])\\
& \rightarrow MLP (512\rightarrow256)
\end{flalign*}
Another max-pooling operation follows to restore the global feature vector and concatenates it to each point. Finally, we obtain our base backbone features $\mathbf{E}\in\mathbb{R}^{N\times 512}$.
\vspace{0.5em}

\noindent\textbf{Initial Flow and Motion Segmentation Head.}
As the base backbone feature $\mathbf{E}$ include complementary features extracted from two input point clouds, we simply use the MLP to implement our initial flow and motion segmentation heads for decoding. The output of the initial flow are 3D flow vectors $\hat{\mathbf{F}}^{init}\in\mathbb{R}^{N\times 3}$:
\begin{flalign*}
& MLP (512 \rightarrow 256\rightarrow 128 \rightarrow 64 \rightarrow 3)
\end{flalign*}
The motion segmentation head estimates per-point moving probabilities $\hat{\mathbf{S}}\in\mathbb{R}^{N}$:
\begin{flalign*}
& MLP (512 \rightarrow 256\rightarrow 128 \rightarrow 64 \rightarrow 1)
\end{flalign*}

\noindent\textbf{Ego-motion Head.} The purpose of our ego-motion head is to derive a rigid transformation $\hat{\mathbf{T}}$ that can summarize the scene flow rigid component induced by the radar ego-motion. To that end, we leverage the differentiable weighted Kabsch algorithm~\cite{kabsch1976solution} that solve the ego-motion estimation problem in a close-form through:
\begin{equation}\label{eq:kabsch}
    \hat{\mathbf{T}}^* = \argmin_{\hat{\mathbf{T}}\in\mathbb{R}^{4\times 4}} \sum_{i=1}^{N} w_i||(\hat{\mathbf{R}}\mathbf{c}_i^{s}+\hat{\mathbf{t}})-\hat{\mathbf{c}}_i^{w}||_2^2
\end{equation}
where ${\mathbf{c}}_i^{w} = \mathbf{c}_i^{s}+\hat{\mathbf{f}}_i^{init}$ is the point coordinates warped by the initial scene flow. The sum of all weights is normalized as $\sum_{i=1}^{N}w_i=1$ and
\begin{equation}
     \hat{\mathbf{T}} = 
     \begin{bmatrix}
     \hat{\mathbf{R}} & \hat{\mathbf{t}}\\
     \mathbf{0} & 1
     \end{bmatrix}
\end{equation}
In our method, we compute the weights from the estimated moving probabilities $\hat{\mathbf{S}}$ via:
\begin{equation}
    w_i = \frac{1-\hat{s}_i}{\sum_{i=1}^{N}{(1-\hat{s}_i)}}
\end{equation}
To solve~\cref{eq:kabsch}, the first step is to compute the centered point coordinates of $\mathbf{C}^{s} = \{\mathbf{c}_i^{s}\}_{i=1}^{N}$ and $\mathbf{C}^{w} =\{\mathbf{c}_i^{w}\}_{i=1}^{N}$. To do that, the weighted centroid of $\mathbf{C}^{s}$ and  $\mathbf{C}^{w}$ can be derived through:
\begin{equation}
    \bar{\mathbf{c}}^{s} = \sum_{i=1}^{N}{w_i\mathbf{c}^{s}_i},\quad
    \bar{\mathbf{c}}^{w} =\sum_{i=1}^{N}{w_i\mathbf{c}^{w}_i}
\end{equation}
We subtract the centroid coordinates from $\mathbf{C}^{s}$ and $\mathbf{C}^{w}$ and obtain the centered point coordinates $\tilde{\mathbf{C}}^{s}\in\mathbb{R}^{N\times 3}$ and $\tilde{\mathbf{C}}^{w}\in\mathbb{R}^{N\times 3}$. A weighted covariance matrix $\mathbf{H}\in\mathbb{R}^{3\times 3}$ can then be formulated as:
\begin{equation}
    \mathbf{H} = \tilde{\mathbf{C}}^{s\top} diag(w_1, w_2, ..., w_N) \tilde{\mathbf{C}}^{w}
\end{equation}
The optimal rotation matrix $\hat{\mathbf{R}}^{*}$ is solved by:
\begin{equation}
    \hat{\mathbf{R}}^{*} = \mathbf{V}
    \begin{bmatrix}
    1 & 0 & 0\\
    0 & 1 & 0\\
    0 & 0 & d\\
    \end{bmatrix}
    \mathbf{U}
\end{equation}
where the singular value decomposition (SVD) is used in $\mathbf{H} = \mathbf{U}\mathbf{\Sigma}\mathbf{V}$ and $d=sign(det(\mathbf{V}\mathbf{U}^{\top}))$ is the correction value to avoid special reflection cases. As the final step, we compute the optimal translation vector as:
\begin{equation}
    \hat{\mathbf{t}}^* = \bar{\mathbf{c}}^{w} - \hat{\mathbf{R}}^{*}\bar{\mathbf{c}}^{s}
\end{equation}

\noindent\textbf{Temporal Update Module.}
This module is embedded in our backbone module and used to propagate information from previous frames when enabled. As a reminder, before we generate our base backbone feature $\mathbf{E}$, we get the feature $\mathbf{L}\in\mathbb{R}^{N\times 256}$ with another multi-scale \emph{set conv} layer. The global feature vector is obtained by $\mathbf{G}\in\mathbb{R}^{256} = MAX(\mathbf{L})$, where $MAX$ is the max-pooling operation along the channel axis. Our temporal update module operates on this global vector $\mathbf{G}$ and applies a GRU network~\cite{cho2014properties} to update it as a hidden state temporally, as seen in~\cref{fig:gru}.

\begin{figure}[tbp!]
    \centering
    \includegraphics[width=0.45\textwidth]{figures/GRU Update.pdf}
    \caption{Temporal update module. We concatenate the updated hidden state $\mathbf{H}$ to each point feature when activating this module, while we use the global feature vector $\mathbf{G}$ directly when the updating module is disabled. Note that the superscript (\eg $l$) denotes the temporal order and we discard it in other places.}
    \label{fig:gru}
\end{figure}

\subsection{Cross-Modal Supervision Details.}
In this sequel, we provide some implementation details on cross-modal supervision mining and loss formulation.
\vspace{0.5em}

\noindent\textbf{Strategy for generate pseudo label $\mathbf{S}^{v}$.}
As introduced in the main text, we propose to generate a pseudo motion segmentation label $\mathbf{S}^{v}$ with the odometry information and radar RRV measurements. As a reminder, the pseudo label $\mathbf{S}^v$ is created by thresholding the ego-motion compensated RRV $\Delta v_i$, \ie object absolute radial velocity. Next, we will discuss our specific thresholding strategy. 

Given per-point $\Delta v_i$, it is intuitive to generate a motion segmentation mask by labeling points with larger values than a fixed threshold as moving points. However, this vanilla strategy suffers from the temporal asynchronization between the well-curated keyframes  and original radar point clouds.  Even though the coordinates of radar points are transformed to the timestamp of keyframes using high-frequency odometry information, their RRV measurements still corresponds to the original timestamps.  As a result, there is often a non-trivial global bias in $\Delta v_i$, which disturbs the identification of real moving points given a fixed threshold. For example, almost all points could be classified as moving when a large bias exists. To mitigate this issue, we propose to normalize all $\Delta v_i$ by subtracting the mean value $\mu$ of them and then classify points by thresholding. The pseudo motion segmentation label $\mathbf{S}^{v}=\{s_i^{v}\in\{0,1\}\}_{i=1}^{N}$ can then be created with a fixed threshold $\eta_v$, where 0 represents stationary points. We determine the value of $\eta_v$ via grid searching on the validation set, as seen in~\cref{fig:direct_thres}. 

To validate if our method helps to improve the quality of pseudo moving labels $\mathbf{S}^v$, we compare this advanced strategy with the direct one. As the pseudo label generation is affected by the threshold $\eta_v$, we change its value by step and observe how the mIoU between the ground truth and pseudo labels vary with the threshold. Fig.~\ref{fig:direct_thres}  shows the comparison between direct thresholding and bias-aware thresholding on the validation set. Without considering the global bias of residuals, direct thresholding can only give a maximum mIoU of 48.40\%, while our proposed bias-aware thresholding produce a mIoU of 52.03\%.  The results demonstrate the effectiveness of our advanced strategy to tackle the temporal misalignment of ego-motion and RRV measurements. Moreover, as shown in the top row, the mIoU increases to a normal level only when the threshold is large enough ($>$ 1.0m/s), which further proves the presence of a global bias in $\Delta v_i$. For the best quality of pseudo label $\mathbf{S}^v$, we set $\eta_v=0.3$ in all our experiments according to the results on the validation set exhibited in Fig.~\ref{fig:direct_thres}.
\vspace{0.5em}

\begin{figure}[tbp!]
    \centering
    \includegraphics[width=0.475\textwidth]{figures/miou_thres_direct.pdf}
    \includegraphics[width=0.475\textwidth]{figures/miou_thres_bias.pdf}
    \caption{The impact of threshold $\eta_v$ when applying direct and bias-aware thresholding to generate pseudo moving labels $\mathbf{S}^{v}$ with ego-motion and RRV measurements. Here, mIoU is computed between the ground truth motion segmentation labels and the generated pseudo labels on the vlidation set.}
    \label{fig:direct_thres}
    \vspace{-1em}
\end{figure}

\noindent\textbf{LiDAR Multi-Object Tracking.}
As another active sensor, LiDAR can detect targets and measure their 3D positions by emitting pulsed lasers~\cite{li2020lidar}. Compared with 4D radar, it can restore the geometric structure well with denser point data under satisfactory weather conditions. Some recent works~\cite{weng20203d,weng2020gnn3dmot,yin2021center} perform 3D multi-object tracking (MOT) on LiDAR point clouds in a \emph {tracking-by-detection} paradigm and show prominent results. Inspired by the progress, we propose to mine supervision signals from LiDAR through running 3D MOT algorithms on LiDAR point clouds. The method we employ is called AB3DMOT~\cite{weng20203d}, which first detects 3D bounding boxes with a pretrained PointRCNN~\cite{shi2019pointrcnn} model and tracks objects based on a 3D Kalman filter~\cite{kalman1960new}. To implement this method, we first use the OpenPCDet\footnote{https://github.com/open-mmlab/OpenPCDet} library and adopt the pretrained PointRCNN model to perform the detection stage. The x, y, z range is [(0, 70.4), (-40, 40), (-3, 1)] meters respectively and the number of points is set as 4096 following the original paper~\cite{shi2019pointrcnn}. For the tracking part, we implement with the official code\footnote{https://github.com/xinshuoweng/AB3DMOT} and take the detection results as the input. Specifically, we set the minimal birth length $Bir_{min}$ as 4 and the maximum death length $Age_{max}$ as 8. The center distance threshold for association is 2 meters. As a result, the 3D MOT algorithm can give us a set of estimated bounding boxes and their IDs at each frame. 
\vspace{0.5em}

\noindent\textbf{Optical Flow Loss.}
Different from LiDAR or radar point
clouds, RGB images contain explicit object appearance and texture information, which provide rich semantics cues for inferring pixel-level 2D motions between frames, \ie optical flow estimation. As a 2D perspective projection of 3D scene flow, optical flow describes the motion of points on the image plane. Thus it can also be used to weakly supervise the scene flow estimation of points, whose perspective projection is within the camera field-of-view (FoV). Thanks to the advance on data-driven optical flow estimation~\cite{teed2020raft,sun2018pwc}, we can use pretrained model to infer pseudo optical flow label efficiently. For one pair of $\mathbf{P}^s$ and $\mathbf{P}^t$, we can input their synchronized monocular images $\mathbf{I}^s$ and $\mathbf{I}^t$ into the network and obtain a optical flow map. We adopt the RAFT-S~\cite{teed2020raft} pretrained model\footnote{https://github.com/princeton-vl/RAFT} to estimate our optical flow. The number of iteration is set as 12 in practice. After aggregating per-point optical flow vectors ${\mathbf{W}}=\{{\mathbf{w}}_i\in\mathbb{R}^2\}_{i=1}^{N}$, we formulate our optical flow loss to constrain our scene flow prediction in the perspective view. In the main text, due to the depth-unawareness during perspective projection, we propose to minimize the point-to-ray distance instead of the flow divergence in pixel scale. Our motivation is further illustrated in~\cref{fig:opt}, where a larger distance between the warped
point $\mathbf{c}^w_j$ and the expected ray $l_j$ results in a smaller pixel-
scale loss after perspective projection for a farther point $\mathbf{c}^s_j$. In particular, we discard the point-to-ray distance lower than 0.25m when computing the loss values to mitigate the impact of optical flow estimation errors.

\begin{figure}[tbp!]
    \centering
    \includegraphics[width=0.475\textwidth]{figures/optical_loss.pdf}
    \caption{Left figure: \textcolor{blue}{Blue} denotes two points (i.e. $\mathbf{c}^s_i$, $\mathbf{c}^s_i$) from the point cloud $\mathbf{P}^1$ and their perspective projection $\mathbf{m}_i,\mathbf{m}_j$ on the corresponding image $\mathbf{I}_s$. \textcolor{red}{Red} arrows denotes pseudo optical flow label $\mathbf{w}_i,\mathbf{w}_j$ and their possible 3D projections (dashing line). Right figure: \textcolor{yellow}{Yellow} denotes the predicted scene flow vectors $\hat{\mathbf{f}_i},\hat{\mathbf{f}_j}$ and their corresponding optical flow after perspective projection. \textcolor{magenta}{Magenta} denotes warped points $\mathbf{c}_i^w, \mathbf{c}_j^w$ and their perspective projection on image $\mathbf{I_s}$. $l_i$ and $l_j$ denotes the corresponding rays of pixels warped by pseudo optical flow labels. }
    \label{fig:opt}
\end{figure}

\subsection{More Experimental Analysis.}

\noindent\textbf{Impact of the Length of Mini-Clips $T$.}
When activating our temporal update module in the backbone, we can update the global feature vector temporally to propagate information from previous frames. However, training with long sequences in a brute-force way will lead to the non-negligible over-fitting. To mitigate the issue, we split long training sequences into many mini-clips with a length of $T$ and train mini-batches of them. During inference, the hidden state is re-initialized after $T$ frames to emulate the training stage. Here, we exhibit how to select the optimal $T$ value in our experiments, as seen in~\cref{tab:update}. As we enlarge the value of $T$, the performance gets improved because temporal information from more previous frames can be used for the current frame. However, when the value of $T$ exceeds 5, the performance starts to degrade and becomes even worse than the one without temporal update when $T=15$. We attribute this to two reasons. First, as we discuss above, longer clips can exacerbate the over-fitting issue. Second, using long-term information from earlier frames will introduce noises and disturb the current feature extraction. 

\begin{table}[htbp!]
    
    \setlength\tabcolsep{8pt}
    \small
    \centering
    \label{modalities}
    \begin{tabular}{lccccccc}
    \toprule
    $T$ & EPE [m]$\downarrow$  & AccS$\uparrow$  &  AccR$\uparrow$ & RNE [m]$\downarrow$  \\
    %& $T$  & EPE [m]$\downarrow$  &  AccR$\uparrow$\\
    \midrule
    1 & 0.1318 & 0.2633 & 0.5517 & 0.0530 \\
    3 & 0.1275 & 0.2795 & 0.5595 & 0.0513\\
    \textbf{5} & \textbf{0.1215} & \textbf{0.2950} &\textbf{0.5792} & \textbf{0.0489}\\
    7 & 0.1306 & 0.2637 & 0.5601 & 0.0526\\
    10 & 0.1289 & 0.2597 & 0.5510 & 0.0519\\
    15 & 0.1417 & 0.2031 & 0.4881 & 0.0571 \\
    \bottomrule
    \end{tabular}
    \caption{Impact of the length of mini-clips for temporal feature update. The results shown above are obtained by evaluating models on the \emph{Val} set. The best $T$ (\textbf{bold}) are used for experiments on the \emph{Test} set.}
    %\todo{Add temporal feature update module to other baselines in the supplementary materials.} }
    \label{tab:update}
\end{table}

\begin{table}[tbp!]
    
    \setlength\tabcolsep{0.5pt}
    \small
    \centering
    \begin{tabular}{lcccc}
    \toprule
    &  \multicolumn{4}{c}{\makecell[t]{\emph{Train (A)}\\\emph{2,409 samples, \textbf{annotated}}}}  \\
    \cmidrule(lr){2-5} 
       Method & ~ EPE [m]$\downarrow$ ~  &  ~ AccS$\uparrow$ ~ & ~ AccR$\uparrow$ ~ &  ~ RNE [m]$\downarrow$ ~ \\
    \midrule
       FlowNet3D~\cite{liu2019flownet3d} &  0.2009 & 0.1685 & 0.3793 & 0.0806  \\
       PointPWC-Net~\cite{wu2020pointpwc} &   0.1959 & {0.1767} & 0.3906 & 0.0786  \\
       FLOT~\cite{puy2020flot} &  0.6023 & 0.0032 & 0.0234 & 0.2413  \\
       FlowStep3D~\cite{kittenplon2021flowstep3d}  & 0.2864 & 0.0610 &	0.1852	& 0.1149\\
       PV-RAFT~\cite{wei2021pv} & \textbf{{0.1256}} & \textbf{{0.2580}} & \textbf{{0.5869}} & \textbf{{0.0506}}	\\
    \midrule
     &  \multicolumn{4}{c}{\makecell[t]{\emph{Train (T)}\\\emph{2,409 samples, \textbf{unannotated}}}}    \\
    \cmidrule(lr){2-5} 
        Method & ~ EPE [m]$\downarrow$ ~  &  ~ AccS$\uparrow$ ~ & ~ AccR$\uparrow$ ~ &  ~ RNE [m]$\downarrow$ ~  \\
    \midrule 
        JGWTF~\cite{mittal2020just} & 0.3853 & 0.0229 & 0.1112 & 0.1544 \\
        PointPWC-Net~\cite{wu2020pointpwc} & 0.3931 & 0.0209 & 0.1089 & 0.1573 \\
        FlowStep3D~\cite{kittenplon2021flowstep3d} & 0.2746 & 0.0358 & 0.1522 & 0.1102 \\
        SLIM~\cite{baur2021slim} & 0.3248 & 0.0520 & 0.1592 & 0.1304 \\
        RaFlow~\cite{ding2022raflow} & 0.2225 & \textbf{0.1885} & 0.3938 & 0.0892 \\
        CMFlow &  {0.1854} & 0.1602 & 0.3888 & {0.0744}  \\
        CMFlow (T) &  \textbf{0.1683} &  {0.1829} &  \textbf{0.4331} &  \textbf{0.0675}  \\
    \bottomrule
    \end{tabular}
    \caption{Comparison between different scene flow methods when keeping the same amount of training samples. Following~\cref{tab:baselines}, fully-supervised methods use the annotated \emph{Train (A)} set for training. Our cross-modal methods and self-supervised baselines train their models on the \emph{Train (T)} set, which can be seen as the unannotated version of the \emph{Train (A)} set.  }
    \label{tab:truncate}
\end{table}

\noindent\textbf{Impact of the Classification Threshold $\eta_b$.}
As a important hyperparameter, $\eta_b$ is used to threshold the estimated moving probabilities $\hat{\mathbf{S}}$ to generate the binary motion segmentation mask during inference, which further determines the flow vectors of which points are refined with the ego-motion estimation. To select its optimal value, we run a series of evaluation on the \emph{Val} set with the trained model and show the results in~\cref{fig:cls_thres}. As we increase the threshold value, the performance on Stat. RNE gets improved continuously, however the optimal threshold for Mov. RNE is 0.5. Considering the scene flow estimation accuracy on both moving and static points are crucial, we aim to seek a trade-off between Stat. RNE and Mov. RNE. We thus set the $\eta_b=0.5$ as the optimal value for our experiments. 

% \begin{figure}[tbp!]
%     \centering
%     \includegraphics[width=0.475\textwidth]{figures/cls_thres.pdf}
%     \caption{Impact of the classification threshold $\eta_b$ on the motion segmentation performance. The value is changed by a step of 0.05.}
%     \label{fig:cls_thres}
%     \vspace{-1em}
% \end{figure}
\begin{figure}[tbp!]
    \centering
    \includegraphics[width=0.475\textwidth]{figures/cls_thres_stat.pdf}
    \includegraphics[width=0.475\textwidth]{figures/cls_thres_mov.pdf}
    \caption{Impact of the classification threshold $\eta_b$ on scene flow estimation. The value is changed from 0.1 to 0.9 by a step of 0.1. }
    \label{fig:cls_thres}
    \vspace{-1em}
\end{figure}

\noindent\textbf{Truncating the {Train} Set.}
For state-of-the-art comparison in~\cref{tab:baselines}, we use more training data ($\sim$2.2k samples) for cross-modal and self-supervised supervised methods than fully-supervised methods. These extra samples do not demand any more collection or annotation efforts since we recycle them from the original test set of~\cite{palffy2022multi}. However, we are interested in how our methods will perform when using the same amount of samples as fully-supervised ones for training. To this end, we truncate the $\emph{Train}$ set here by removing the extra samples and name the truncated unannotated one as the $\emph{Train (T)}$ set. We train our methods and self-supervised baselines on this truncated set and compare them with fully-supervised methods that use the annotated $\emph{Train (A)}$ for training. The results are shown in~\cref{tab:truncate}. Even after truncating our \emph{Train} set, our cross-modal supervised method still shows competitive results compared with state-of-the-art supervised methods. It is interesting to find that our methods have a  lower AccS than the self-supervised RaFlow~\cite{ding2022raflow} method. We explain this by the fact that self-supervised scene flow methods only exploit the input itself to constrain the predictions and thus need less samples to be trained well. However, when we use the original \emph{Train} set, our methods perform much better than all self-supervised methods on different metrics.
